# Supplementary material for: Interaction between two overall neutral charged microscopically patterned surfaces
Source: arXiv:2307.04650 source file (2023-07-10)
Supplement: Supplementary file 1 [file 2015-SM-Sidney-crittical-adsorption-confinement-v.11.pp._4430-4443.pdf]

Soft Matter

PAPER

View Article Online
View Journal | View Issue

Published on 22 April 2015. Downloaded by UNIVERSITATSBIBLIOTHEK POTSDAM on 27/05/2015 10:41:52.

Cite this: *Soft Matter*, 2015, **11**, 4430

# Inverted critical adsorption of polyelectrolytes in confinement†

Sidney J. de Carvalho,*[a] Ralf Metzler[bc] and Andrey G. Cherstvy[c]

What are the fundamental laws for the adsorption of charged polymers onto oppositely charged surfaces, for convex, planar, and concave geometries? This question is at the heart of surface coating applications, various complex formation phenomena, as well as in the context of cellular and viral biophysics. It has been a long-standing challenge in theoretical polymer physics; for realistic systems the quantitative understanding is however often achievable only by computer simulations. In this study, we present the findings of such extensive Monte-Carlo *in silico* experiments for polymer–surface adsorption in confined domains. We study the inverted critical adsorption of finite-length polyelectrolytes in three fundamental geometries: planar slit, cylindrical pore, and spherical cavity. The scaling relations extracted from simulations for the critical surface charge density $\sigma_c$—defining the adsorption–desorption transition—are in excellent agreement with our analytical calculations based on the ground-state analysis of the Edwards equation. In particular, we confirm the magnitude and scaling of $\sigma_c$ for the concave interfaces *versus* the Debye screening length $1/\kappa$ and the extent of confinement $a$ for these three interfaces for small $\kappa a$ values. For large $\kappa a$ the critical adsorption condition approaches the known planar limit. The transition between the two regimes takes place when the radius of surface curvature or half of the slit thickness $a$ is of the order of $1/\kappa$. We also rationalize how $\sigma_c(\kappa)$ dependence gets modified for semi-flexible *versus* flexible chains under external confinement. We examine the implications of the chain length for critical adsorption—the effect often hard to tackle theoretically—putting an emphasis on polymers inside attractive spherical cavities. The applications of our findings to some biological systems are discussed, for instance the adsorption of nucleic acids onto the inner surfaces of cylindrical and spherical viral capsids.

Received 17th March 2015, Accepted 15th April 2015

DOI: 10.1039/c5sm00635j

www.rsc.org/softmatter

## I. Introduction

The adsorption of charged polymers or polyelectrolytes (PEs) onto oppositely charged surfaces[1–5] has a number of technological and biophysical applications including paper production,[8,9] interface coating,[10] layer-by-layer formation,[6,7] water desalination,[11,12] and stabilization of colloidal suspensions.[13,14] One distinguishes weak and strong PE–surface adsorption:[5] weak PE–surface adsorption is governed by an interplay of energetic often electrostatic (ES) attraction of polyions onto an interface *versus* an entropic penalty accompanying the confinement[15,16] or the compression of the polymer chains near the surface.[17–19] Weak adsorption takes place for weakly charged PEs (partially neutralized by condensed counterions[20,21]) and for moderately charged interfaces: such PE–surface binding is rather reversible. This contrasts an irreversible adsorption in the limit of strong PE–surface association.[5,22]

Weak PE adsorption onto surfaces of different geometries at varying conditions has been investigated in a number of recent theoretical,[5,23–42] experimental,[43–58] and computer simulation[59–78] studies. PE adsorption onto patterned and corrugated surfaces[32,33,79–83] as well as critical PE adsorption onto charged Janus net-neutral particles[59] was also examined. The properties of polymer adsorption inside cylindrical nanopores in porous glass were studied experimentally and by computer simulations in ref. 44. Possible effects of surface dielectric discontinuities on PE–surface adsorption were rationalized too.[84–86]

The critical adsorption describes the threshold conditions at which the ES-driven adsorption of PE chains first takes place in the system. This phase transition interrelates the condition for the interface surface charge density $\sigma$, the line charge density of the polymer $\rho$, the reciprocal Debye screening length in the solution $\kappa$, the ambient temperature $T$, and the polymer's Kuhn length $b$. The critical adsorption condition defines the relation between these important model parameters at the

[a] *Institute of Biosciences, Letters and Exact Sciences, Sao Paulo State University, 15054-000 Sao Jose do Rio Preto, Brazil. E-mail: sidneyjc@ibilce.unesp.br*
[b] *Department of Physics, Tampere University of Technology, 33101 Tampere, Finland*
[c] *Institute for Physics & Astronomy, University of Potsdam, 14476 Potsdam-Golm, Germany. E-mail: rmetzler@uni-potsdam.de, a.cherstvy@gmail.com*

† Electronic supplementary information (ESI) available. See DOI: 10.1039/c5sm00635j

 This journal is © The Royal Society of Chemistry 2015

Published on 22 April 2015. Downloaded by UNIVERSITATSBIBLIOTHEK POTSDAM on 27/05/2015 10:41:52.

coexistence boundary of adsorbed *versus* desorbed chain conformations. Typically, a universal critical adsorption parameter can be constructed,

$$\delta_c = \frac{24\pi a^3|\rho\sigma_c|}{\varepsilon k_B T b}, \tag{1}$$

and its dependence on $\kappa$ governs the scaling of $\sigma_c$—the critical surface charge density required for PE adsorption to take place—at varying salt conditions. Here $\varepsilon$ is the dielectric constant of the medium, $a$ is the curvature radius of the adsorbing surface, and $k_B$ is the Boltzmann constant. For a long flexible nearly Gaussian charged polymer in front of a uniformly oppositely charged plane the well-known result is[17,18,26]

$$\delta_c^{pl}(\kappa) \sim \sigma_c^{pl}(\kappa) \sim \kappa^3. \tag{2}$$

The standard rationale for increasing $\sigma_c$ with the salt concentration $n_0$ is the requirement to compensate a stronger screening of ES attraction of the PE chain to the oppositely charged surface. For a symmetric 1 : 1 electrolyte we have $\kappa^2 = 8\pi l_B n_0$, where $l_B = e_0^2/(\varepsilon k_B T)$ is the Bjerrum length. The peculiar cubical scaling of the critical charge density with $\kappa$ in eqn (1) stems from the properties of the eigenfunctions of the corresponding Edwards equation for polymer conformations in the attractive Debye–Hückel potential of the interface.[17] In addition, some ES chain stiffening at low-salt conditions takes place impeding the PE–surface adsorption (see also ref. 34 for non-ES effects in PE–surface adsorption).

For the convex cylindrical geometry (see Fig. 1) a quadratic scaling is instead predicted by the Wentzel–Kramers–Brillouin (WKB) theory at low salt,[38] namely

$$\delta_c^{cyl}(\kappa a) \sim (\kappa a)^2, \tag{3}$$

while at high salinities and large rod radii $\kappa a \gg 1$ the planar limit (2) is recovered. For PE adsorption on the outside of oppositely charged spherical particles the theory yields the linear dependence of $\sigma_c(\kappa a)$ in the limit $\kappa a \ll 1$,[38]

$$\delta_c^{sp}(\kappa a) \sim (\kappa a)^1. \tag{4}$$

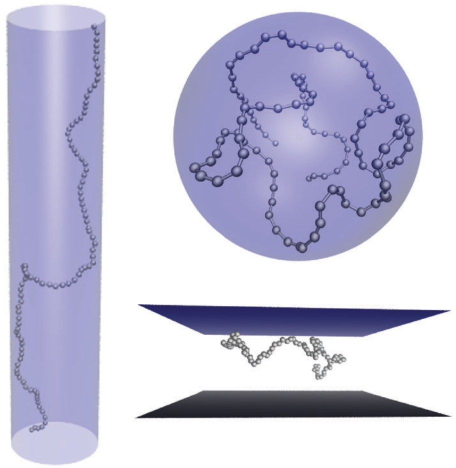

Fig. 1 Schematics of the inverted PE adsorption in confinement: planar slit, cylindrical pore, and spherical cavity. Video files illustrating the conformational changes of the polymer chain for conditions below and above the critical adsorption transition are presented in the Supplementary material.

Here $a$ is the radius of the cylinder or sphere. The prefactors in these WKB scaling relations are very close to the exact analytical results available *e.g.* for the planar and spherical surfaces.[38] For more details on these scalings we refer the reader to ref. 5, 38 and 59.

The systematic change in the $\sigma_c(\kappa a)$-scaling behavior from the planar interface *via* a cylinder to a sphere is in agreement with a number of experimental results from the Dubin's lab, see *e.g.* ref. 47 (and also the analysis in ref. 36). The experimental observations of critical PE adsorption are based on the complex formation of various polymers with oppositely charged particles and micelles of spherical and cylindrical geometry.[47] These experimental findings indicate a weaker dependence of $\sigma_c$ on $\kappa a$ for more "convex" surfaces, as the adsorbing interfaces transfer from the planar to the cylindrical and finally to the spherical shape.

The adsorption transition of weak PEs under confinement[31]—we call below the inverted critical adsorption—has a number of biologically relevant applications. Here, the term critical for confined PEs has the same meaning as for adsorption of charged polymers onto planar and convex interfaces.[5] For instance, the self-assembly of cylindrical and spherical single-stranded RNA viruses involves the adsorption of nucleic acids onto the inner virus capsid surface composed of protein building blocks.[29,40,41,87,88] The capsid proteins are abundant in highly basic flexible polypeptide tails which trigger the adsorption of negatively charged nucleic acids thus steering the self-assembly.[89,90] The known examples include nucleic acid encapsulation inside the cylindrical tobacco mosaic virus (TMV)[91] and the icosahedral cowpea chlorotic mottle virus (CCMV).[29,92,93]

For very long chains, the scaling relations for critical PE adsorption in inverted geometries were recently derived theoretically from the ground-state analysis of the Edwards equation for the Green function.[39] The main subject of the current paper is the inverted weak adsorption of finite-length PE chains of varying stiffness in all three basic geometries (see Fig. 1). For long flexible polymers near planar and convex surfaces the critical adsorption conditions were obtained using the WKB method in ref. 38. Namely, eqn (5)–(7) of ref. 38 provide the dependence of $\sigma_c$ in the entire range of $\kappa a$. At low salt or strong confinement (when $\kappa a \ll 1$) the critical adsorption parameter $\delta_c^{inv}$ for a planar slit was predicted to scale as[39]

$$\delta_c^{pl,inv} \sim 3C^2(\kappa a)^1. \tag{5}$$

Here and below the constant $C$ is of order unity, $C \approx 0.973$. For long flexible PEs inside the oppositely charged cylinder this parameter reveals a plateau with a slowly varying logarithmic correction[39]

$$\delta_c^{cyl,inv} \sim \frac{3C^2}{0.116 - \log(\kappa a)}. \tag{6}$$

Published on 22 April 2015. Downloaded by UNIVERSITATSBIBLIOTHEK POTSDAM on 27/05/2015 10:41:52.

Finally, for a PE inside spherical cavities in the low salt limit the value of $\delta_c$ tends to saturate to a plateau[39]

$$\delta_c^{sp,inv} \sim 3C^2. \quad (7)$$

These functional dependencies on $\kappa a$ are in stark contrast to the fast and monotonically increasing $\delta_c$ for the adsorption of PEs on the outside of cylindrical and spherical interfaces (eqn (3) and (4)). In the opposite limit of loose confinement or high salt (when $\kappa a \gg 1$) the theory predicts

$$\delta_c^{inv} = 3C^2(\kappa a)^3/2 \quad (8)$$

for all three inverted geometries.[39] This latter limiting behavior was derived from the WKB approach in the limit of zero surface curvature.[5,38] Note that for a finite-length polymer all the above mentioned standard ground-state based predictions for $\sigma_c$ need to be modified; the regular procedure is however not easy. Also, in theory the polymer chain is treated at the mean-field level in terms of the probability distribution function, with no explicit examination of polymer loops or tails on the surface being possible. These facts make the findings of our current computer simulations—which enable us to overcome these theoretical limitations—even more valuable for experimentally relevant situations.

In the current paper we study by extensive Monte-Carlo simulations the properties of critical PE adsorption in three basic inverted geometries (see Fig. 1). We study the effects of the chain length, the polymer persistence, and systematically of the confinement size and solution salinity on the critical surface charge density $\sigma_c$. In Section II we present the details of the simulation model and the data analysis algorithms. The main results on PE adsorption profiles and critical adsorption characteristics are described in Section III. We discuss the physical rationales behind the observed dependencies and the applications of our results in Section IV.

## II. Model and approximations

We here implement the same Metropolis Monte-Carlo simulation algorithm which has been successfully applied and tested by us recently for PE adsorption onto spherical,[64] cylindrical,[61] and spherical Janus[59] particles as well as for surface adsorption of pH-sensitive PEs.[65] We refer the reader to ref. 59, 61 and 64 for more details on the simulation procedure. In brief, the polymer chain is modeled within the spring-bead model, with each monomer being a rigid sphere of radius $R_m$ = 2 Å carrying a point elementary charge $Z_m = e_0$ at its center. Neighboring beads are connected by the harmonic potential

$$U_{str}(r) = K_r(r - r_0)^2/2,$$

with the elastic constant for bond stretching $K_r$ = 1.0 N m$^{-2}$ and the inter-monomer equilibrium distance $r_0$ = 7.0 Å (as for single-stranded DNA[96]). The chain stiffness is given by the elastic potential

$$U_{el}(\theta) = K_\theta(\theta - \theta_0)^2/2,$$

where the force constant $K_\theta$ assumes the values such that the non-ES persistence length $l_{p,0}$ of the polymer ranges from about 8 to 50 Å (a typical range for many real PEs[5]). Here $\theta$ denotes the angle between the two successive bonds and $\theta_0 = \pi$. The mechanical persistence length $l_{p,0}$ was obtained in simulations *via* the relation $l_{p,0} = \langle R^2\rangle^{1/2}/(1 + \langle\cos\theta\rangle)$, where $\langle R^2\rangle$ is the root-mean-squared monomer–monomer distance.[97] The inter-chain excluded volume is accounted for by the standard hard-core repulsive potentials in simulations, as compared to the theoretical model.[39]

The repulsion of monomers at distance $r$ is given by the screened Coulomb potential

$$U_{ES}(r) = \frac{Z_m{}^2 e^{-\kappa r}}{\varepsilon r}. \quad (9)$$

The ES potentials emerging in a slit with inter-plane distance $2a$, inside a cylinder or a sphere of radius $a$, were computed as the solutions of the linear Poisson–Boltzmann equation.[39] Below, we use the potentials denoted as $\Psi_{in,out}(r)$ in ref. 39 to parametrize the strength of ES PE–surface attraction. For brevity, we do not provide the explicit analytical expressions here, instead showing the potential distributions in Fig. 2.

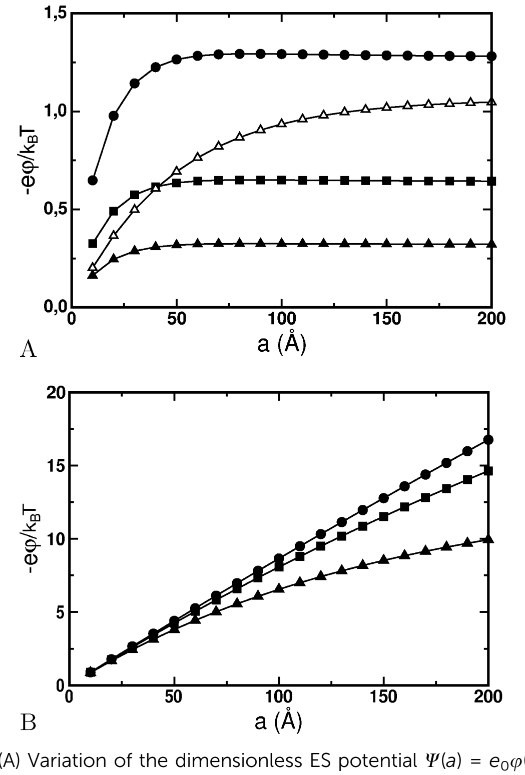


Fig. 2 (A) Variation of the dimensionless ES potential $\Psi(a) = e_0\varphi(a)/(k_BT)$ at the boundary *versus* the radius of the spherical cavity plotted for $\sigma = -0.1/(4\pi)$ C m$^{-2}$ and $\kappa$ = 1/(30 Å) (filled circles), $\sigma = -0.1/(8\pi)$ C m$^{-2}$ and $\kappa$ = 1/(30 Å) (filled squares), $\sigma = -0.1/(16\pi)$ C m$^{-2}$ and $\kappa$ = 1/(30 Å) (filled triangles), and $\sigma = -0.1/(16\pi)$ C m$^{-2}$ and $\kappa$ = 1/(100 Å) (empty triangles). Note that C m$^{-2}$ $\approx e_0/(16$ Å$^2)$ that is $\approx 6\sigma_{B\text{-}DNA}$, where $\sigma_{B\text{-}DNA}$ is the bare charge density of the B-DNA.[96] For large $a$ values the potential approaches the known planar result, $\varphi(a) = 4\pi\sigma/(\varepsilon\kappa)$. (B) The ES potential on the inner surface of spherical cavities scales as $\Psi(a) \sim \kappa a$ for $\kappa a \ll 1$, whereas $\Psi(a) \to e_0\varphi(a)/(k_BT)$ for $\kappa a \gg 1$. Parameters: $\sigma = -0.1/(4\pi)$ C m$^{-2}$, $\kappa$ = 1/(3000 Å) (filled circles), $\kappa$ = 1/(1000 Å) (filled squares), and $\kappa$ = 1/(300 Å) (filled triangles).

Published on 22 April 2015. Downloaded by UNIVERSITATSBIBLIOTHEK POTSDAM on 27/05/2015 10:41:52.

The critical surface charge density $\sigma_c$ is defined in our simulations as the condition at which the PE binding energy to the interface exceeds the thermal energy,

$$|E_b| \geq k_BT. \tag{10}$$

Thus, even for the conditions when the polymer is not in direct contact with the surface but its total binding energy is lower than $E_b = -k_BT$, we consider the chain to be in the adsorbed state. To compute the value of $\sigma_c$ for given values of the model parameters $\kappa$, $a$, and $N$, we perform the simulations for a set of surface charge densities and then determine the one for which the adsorption–desorption criterion (10) is satisfied. Here one can anticipate already that longer chains will require smaller surface charge densities $\sigma_c$ to be classified as adsorbed, as we indeed obtain from simulations (see below and also ref. 98). In the limit $a \to \infty$ the potentials $\Psi_{in,out}(r)$ of ref. 39 turn into $\Psi(r)$ for the corresponding isolated surfaces (see Fig. 2); the same holds for the properties of the adsorption–desorption transition (see below).

There exist a number of differences between the inverted PE adsorption and the polymer–surface adsorption from a dilute, free-space solution. One feature is the presence of confining interfaces. They have different implications for the polymer: for a planar slit the polymer is mobile in two dimensions, for a cylindrical tube the chain is free to move in one direction, and for a spherical cavity the polymer has no translational freedom at all. This progressively increasing confinement reduces the polymer conformational entropy,[99] particularly upon adsorption on the interior of oppositely charged cylinders and spheres (see also ref. 100).

We also note that in the low-salt limit the total PE persistence length,

$$l_p(\kappa) = l_{p,0} + l_p^{ES}(\kappa) = b/2, \tag{11}$$

acquires an ES component decreasing with the solution salinity. For flexible chains it obeys the scaling $l_p^{ES}(\kappa) \sim \kappa^{-1}$ (ref. 2) while for semi-flexible polymers $l_p^{ES}(\kappa) \sim \kappa^{-2}$ (ref. 1, see also ref. 101–105). This fact is not accounted for in the theories of PE–surface adsorption[38,39] yielding for $\delta_c^{inv}$ the scaling relations (5)–(7). This ES contribution $l_p^{ES}$ should correspondingly renormalize the scaling of $\sigma_c$ with $\kappa$ obtained from computer simulations at low salt, in accord with eqn (1) (see the discussion in ref. 5 and also ref. 18 for planar and convex surfaces). For concave adsorbing interfaces, such as the sphere's inner surface, due to this ES polymer stiffening the chains will tend to occupy regions of smaller curvature,[99] as it is indeed observed upon "spooling" of double-stranded DNA inside bacteriophages.[106] The chains approach the interface because of bending energy minimization, thus facilitating the ES-driven PE–surface binding (see below).

An additional important parameter for confined PE–surface adsorption is the polymer's volume density. In theory[5,38] the PE adsorption typically takes place from a very dilute polymer solution, which is not the case for confined inverted-adsorption situations, where the net polymer density is finite (see below).

Let us now briefly discuss some approximations involved in the current study.

(a) We use the Debye–Hückel theory to compute the ES potentials near the interfaces and between the polymer monomers. This approach is valid for weakly charged systems and for an appreciable amount of salt in the solution $n_0$, when the ES potentials $|\Psi| \leq 25$ mV (compare the panels of Fig. 2). The solution of the nonlinear Poisson–Boltzmann equation in curved geometries in the presence of salt is a formidable theoretical problem per se, often only solvable in some idealized limits (see ref. 107 for a charged rod at $n_0 = 0$). Note that the linear ES theory often overestimates the magnitude of the potential emerging near highly charged interfaces (see Fig. 2 of ref. 108 and 109). Also note that particularly in low-salt solutions, the effects of counterion release from the surface upon PE adsorption[110–112]—at the level of the standard Poisson–Boltzmann approach with the cation concentration obeying $n(\mathbf{r}) = n_0e^{-\Psi(\mathbf{r})}$ and beyond—might become relevant.

(b) The WKB scaling relations presented in the Introduction stem from the ground-state analysis of infinitely long flexible Gaussian chains in front of surfaces with the Debye–Hückel ES potential. Both these idealizations will not hold upon variation of $n_0$ in a broad range, as we study below. The implications of the non-linear nature of the ES potential near highly charged surfaces is the subject of a separate investigation.[113] Also, the mutual influence of adsorbing PE chains on the ES potential of the interface (charge regulation) can non-trivially impact the critical adsorption conditions in terms of $\sigma_c(\kappa)$ scaling. Moreover, we consider below the adsorption of a single PE chain from a dilute solution; under realistic conditions however several chains might adsorb simultaneously. Their mutual salt-dependent ES repulsion along the surface will have an effect, for instance, on the overall surface coverage by PEs. The latter is often measured experimentally for PE–surface adsorption from bulk solutions with a finite polymer concentration. All these effects are experimentally relevant and will be considered elsewhere.[113]

(c) We implement the physically intuitive $k_BT$-based adsorption criterion (10) to identify the PE adsorption–desorption threshold. This criterion was used *e.g.* in computer simulations[76] and experimental studies of formation of PE–protein complexes.[46] Such a criterion for confined adsorption is however somewhat arbitrary: for instance, one can classify the adsorption threshold using PE distributions with a single peak *versus* the double-peaked profiles emerging between the two confining interfaces (see *e.g.* Fig. 3). Note here that there exists a conceptual difference between PE adsorption from the empty space and inside a confined cavity. For the former, counting the chain configurations in the course of simulation one can clearly distinguish the desorbed state with zero binding energy and the adsorbed state with the adsorption energy of several $k_BT$ units.[59,61] This phase transition line then determines the first-order transition boundary. Then, the polymer chain staying for $>50\%$ of the simulation time in adsorbed configurations is considered to be in the adsorbed state. For the polymer adsorption under *e.g.* spherical confinement this procedure is no longer

Published on 22 April 2015. Downloaded by UNIVERSITATSBIBLIOTHEK POTSDAM on 27/05/2015 10:41:52.

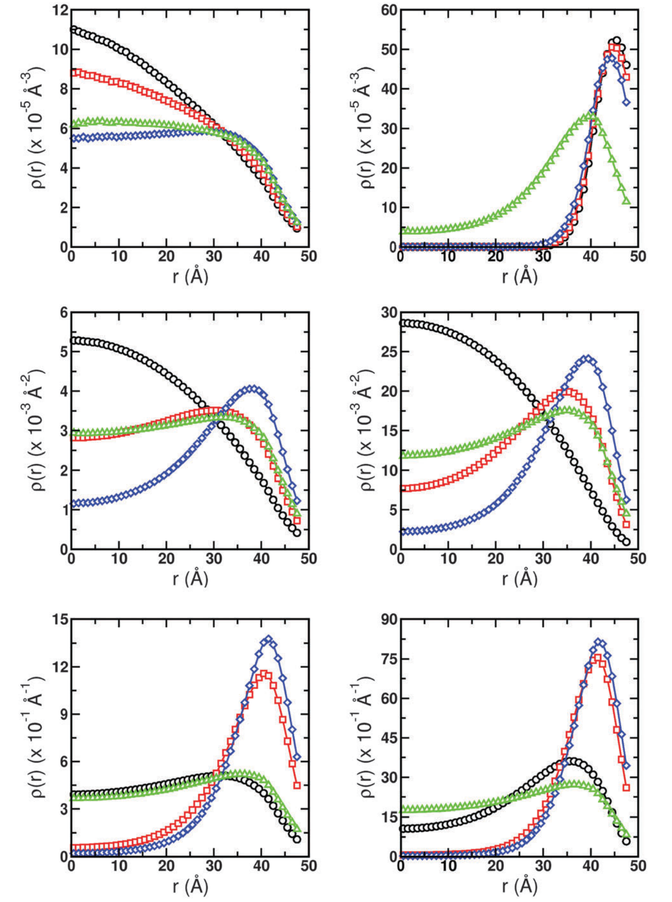


Fig. 3 Distribution of polymer monomers for inverted adsorption of flexible PEs ($l_{p,0}$ = 8 Å) in a spherical cavity (top panels), cylindrical pore (middle panels) and planar slit (bottom panels) with the surface charge density of $\sigma = -0.1/(4\pi)$ C m$^{-2}$. The radius of the sphere and cylinder is $a$ = 50 Å, and the slit thickness is $2a$ = 100 Å. The distance $r$ denotes the separation from the centre of the confining space. The polymer density distribution $\rho(r)$ used here is not to be mixed with the PE linear charge density $\rho$. The degree of chain polymerization is $N$ = 20 (left panels) and $N$ = 100 (right panels). The salt concentration $n_0$ is varied: $\kappa a$ = 0.1 (black), $\kappa a$ = 0.5 (red), $\kappa a$ = 1 (blue) and $\kappa a$ = 5 (green symbols).

possible: the well-defined energy-separated states of the polymer near the surface do not exist (in general sense, no first-order-like transition, see Fig. 8). This was the reason to use another adsorption criterion here as compared to PE adsorption problems treated in ref. 59, 61 and 64.

(d) We assume reversibility and ergodicity[114] for the process of PE adsorption under all conditions (no irreversible binding). This assumption might not be valid, particularly at low salt when the binding of even several PE monomers to an interface with a large ES potential might overcome the thermal energy. Also, in this limit the relative accuracy in defining the adsorption–desorption boundary becomes important and even small fluctuations $|\delta\sigma_c|/|\sigma_c|$ that can realize in experiments might cause sizable effects. Finally, the adsorption of one fragment of the chain is assumed not to affect the ES potential acting to attract other parts of the polymer. This might be important for pH- and potential-responsive surfaces (not a part of this study[113]). We work in the single-chain limit and thus do not study the PE adsorption isotherm—the amount of polymer adsorbed for a varying bulk polymer concentration. The experimentally more relevant situation of multi-chain adsorption is a subject of separate investigation (see some results in Fig. 4B). The multi-chain effects are extremely important to determine *e.g.* the amount of PE adsorbed per unit surface area. This issue should include additional approaches/models for computing the steric and ES effects of neighboring chains as well as the effective charge density of the interface which is partially covered with already adsorbed PE chains.

Despite these simplifications and assumptions, our computational results reveal excellent agreement with the theoretical predictions in a wide range of model parameters (see below).

# III. Results

## A. Polymer density distribution

First, we examine the distribution of polymer monomers, $\rho(r)$, in the three basic inverted geometries. For a fixed degree of the external confinement, the evolution of the $\rho(r)$ profiles with varying $n_0$ reflects the positioning of the adsorption–desorption boundary. We start with relatively flexible chains confined to a spherical cavity and a cylindrical pore; we use $l_{p,0}$ = 8 Å for flexible chain results below. If the unperturbed radius of gyration of the chain exceeds the cavity dimensions, $\sqrt{\langle R_g^2 \rangle} \gtrsim a$, volume exclusion creates a force pushing the polymer towards the surface (see Fig. 3). This is particularly pronounced for spherical cavities, with strongly restricted chains. With increasing ionic strength up to $\kappa a$ = 1 the monomer accumulation near the surface gets facilitated. From $\kappa a$ = 1 to $\kappa a$ = 5 this behavior gets inverted, as at large $\kappa a$ the conditions are close to or above the threshold of polymer desorption, and in addition the ES term in the chain persistence length gets smaller. This makes the polymer chains effectively more flexible, they are attracted weakly to the interface, and the polymers occupy the bulk of the cavity more readily. In this situation we thus find a single peak of the polymer distribution in the centre of the confining space, whereas for small $\kappa a$ the PE peak emerges near the oppositely charged surface in confined geometries, see Fig. 3.

The effect of polymer's mechanical persistence on PE distribution in confined spaces is illustrated in Fig. 9. Progressively stiffer PE chains prefer to occupy the peripheral regions of the cavity due to a lower bending energy penalty for the chain arrangements with larger radii of curvature – the effect is particularly pronounced for spherical cavities (see the top row in Fig. 9). These latter trends are in line with the results of our recent simulations for polymer chains inside inert or non-attractive spherical cavities in the presence of macromolecular crowding[99] (see also ref. 115 and 116). Moreover, the loss of configurational entropy for the arrangement of more persistent chains near the cavity surface is smaller as compared to the flexible ones. Fig. 9 shows that the deviations for semi-flexible *versus* flexible chains become smaller as we go from PE adsorption inside a spherical cavity to PE adsorption inside a cylindrical

 This journal is © The Royal Society of Chemistry 2015

Published on 22 April 2015. Downloaded by UNIVERSITATSBIBLIOTHEK POTSDAM on 27/05/2015 10:41:52.

pore and finally to PE adsorption inside a planar slit (respectively, the top, middle and bottom panels of Fig. 9). The physical reason is again the number of polymer's degrees of freedom available in the corresponding geometries. For instance, for a planar slit the bending energy of semi-flexible chains has nearly no implications for the amount of the polymer near the adsorbing interface, in stark contrast to the spherical cavity for which a severe chain bending is unavoidable[99] (compare the panels in Fig. 9). As we demonstrate below, this polymer bending energy in spherical and cylindrical confinement has non-trivial effects on the critical surface charge density $\sigma_c(\kappa a)$ of the adsorption–desorption transition.

A relevant experimental question for super-critical PE adsorption is the amount of the polymer adsorbed on the surface. In Fig. 4 we quantify how this amount changes with $\kappa a$ for the three adsorption geometries for the single-chain adsorption simulation. Namely, for $\sigma > \sigma_c$ we analyzed the PE profiles formed near the interfaces for the inverted polymer adsorption. We evaluate the fraction of the polymer chain in the region close to the adsorbing interface, $N_{ads}/N$. This fraction is a stationary quantity: we do not consider here the kinetics of PE adsorption for $\sigma > \sigma_c$[2,78,117,118] and the total time required to complete the adsorption. We illustrate the behavior of this fraction *versus* the reciprocal Debye screening length $\kappa$ for two different chain lengths of $N$ = 20 and $N$ = 100 monomers (see Fig. 4A and B respectively). To quantify the effects of the chain length, in Fig. 4B we also show the data for adsorption of five $N$ = 20 chains inside a spherical cavity. The fraction of monomers adsorbed $N_{ads}/N$ is found to be quite close to that computed for a single chain with $N$ = 100 monomers.

We find that the amount of PE adsorbed within this first layer near the interface is often a non-monotonic function of the salt concentration $n_0$. One physical reason for this is a shorter ES persistence length of PEs and weaker polymer–surface charge-mediated binding as $n_0$ increases. This non-monotonicity can be anticipated already from the evolution of PE profiles in Fig. 3 in the proximity of the adsorbing surface as $\kappa$ increases. Here, we refer the reader to the studies in ref. 34 and 48 for experimental evidence and theoretical predictions of non-monotonic effects of added salt on the amount of adsorbed PE chains. In realistic multi-chain systems, higher solution salinities effect softer PE chains, weaker PE–surface ES attraction, but also a weaker ES repulsion between the already adsorbed polymer coils. The interplay of these effects might yield a non-monotonic behavior of the mass-per-area of adsorbed PEs with varying $\kappa$. Fig. 4C quantifies the growth of the fraction of adsorbed PE monomers for the chains of varying length inside a spherical cavity. The results are plotted for different values of $\kappa$. As expected, we observe that for longer chains low-salt conditions give rise to a stronger PE adsorption, with a larger $N_{ads}/N$ fraction.

The width of the PE profile $w$ and the mass of adsorbed PE per area are the experimentally relevant quantities to measure the deposition propensity of the polymer onto a surface. As we work in the single chain limit, the latter will not be considered. For inverted PE adsorption, the width of the adsorbed layer is expected to be a non-monotonic function of $\kappa$ too. Note however that the standard definition of $w$ implemented for instance for the adsorption of an isolated PE chain onto an attractive surface[5]—as the width of the polymer probability distribution function at its half-height—cannot be directly used for the current problem of inverted adsorption.

### B. Critical adsorption conditions

Now we turn to the main objective of the current study, the scaling of the critical surface charge density at the adsorption–desorption transition. For the inverted PE adsorption in confined geometries, we find that $\sigma_c$ varies with $\kappa a$ as shown in Fig. 5, revealing an excellent agreement with the theory developed in ref. 39. As expected, the scaling of the critical surface charge density is very different in the limit of small and large $\kappa a$ values, as prescribed by eqn (5)–(8), respectively. In the low-salt limit spherical cavities necessitate larger surface charge densities than the cylindrical tubes; the latter in turn need larger surface charges than the planar slits in order to reach the same degree of polymer binding (10) (compare the curves in Fig. 5). We attribute this reduction of $\sigma_c^{inv}$ to a progressively smaller penalty of entropic confinement of flexible PE chains. Remarkably, even the reversed order of the critical adsorption

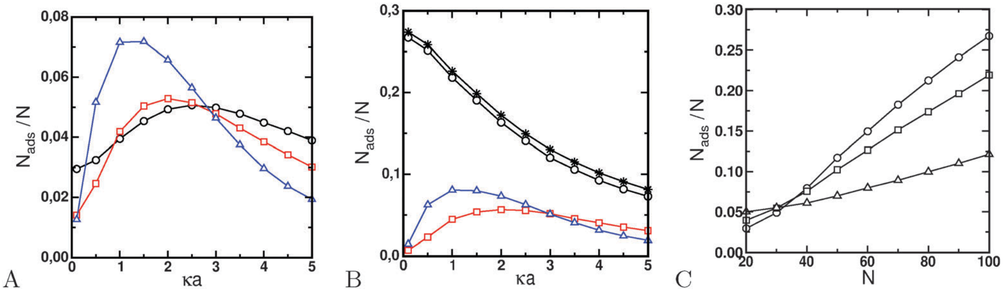


Fig. 4 Fraction of polymer monomers within 4 Å from the adsorbing surface for inverted PE adsorption into a spherical cavity (black), cylindrical pore (red) and planar slit (blue symbols) with $\sigma = -0.1/(4\pi)$ C m$^{-2}$ (above the critical adsorption transition), plotted for a varying solution salinity. The radius of the spherical cavity and the cylindrical tube is $a$ = 50 Å and the inter-plane distance for the slit is $2a$ = 100 Å; $N$ = 20 (panel A) and $N$ = 100 (panel B); $l_{p,0}$ = 8 Å. The results for five $N$ = 20 chains are denoted by star symbols in panel B. Panel C shows the variation of the adsorbed PE fraction in a spherical cavity with the polymerization degree $N$, computed for the same $\sigma$, $l_{p,0}$, $a$ values for varying salt conditions, namely at $\kappa a$ = 0.1 (circles), 1 (squares), and 3 (triangles).

Published on 22 April 2015. Downloaded by UNIVERSITATSBIBLIOTHEK POTSDAM on 27/05/2015 10:41:52.

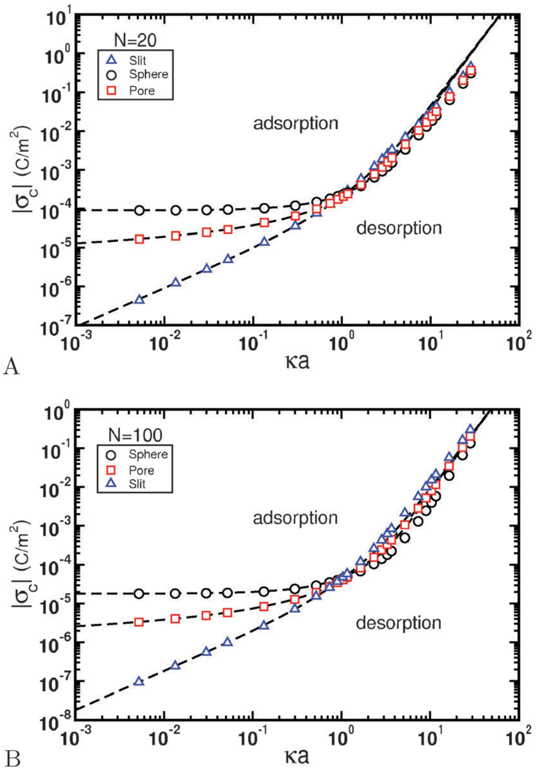


Fig. 5 Critical surface charge density $\sigma_c$ for inverted adsorption of flexible PEs ($l_{p,0}$ = 8 Å) into a planar slit (blue symbols), cylindrical tube (red symbols), and spherical cavity (black symbols), plotted for varying solution salinity. The dashed lines are the full theoretical asymptotes for $\delta_c$ as given by eqn (7) in ref. 39, recalculated for $\sigma_c$ using eqn (12). The corresponding low-salt limits are given by eqn (5)–(7); the high-salt or the planar limit is eqn (8). Note the inverse positioning of the curves in the region of $\kappa a \gg 1$. Parameters: $a$ = 50 Å (1/2 of the slit thickness, the cylinder and sphere radii), the polymerization degree is $N$ = 20 (panel A) and $N$ = 100 (panel B). On a standard 3–3.5 GHz workstation every curve on these graphs requires some 180 h and 900 h of computational time for chains of $N$ = 20 and $N$ = 100 monomers, respectively.

curves in the limit of large $\kappa a$, as compared to the low-salt limit, is precisely reproduced in our simulations, in accord with the theory.[39] This reversed order at high salt is particularly well pronounced for longer chains (Fig. 5B). The change in the $\sigma_c(\kappa a)$ scaling behavior, from the low-salt prediction to the high-salt asymptote (8), occurs at $\kappa a \sim 1$, for any chain length (compare the panels in Fig. 5). The effects of the surface curvature on the adsorption–desorption transition point are thus universal and start to be important for the conditions of low-salt and large surface curvature when $\kappa \lesssim 1/a$. Fig. 5 is the central result of the current study.

For progressively longer PE chains the values of $\sigma_c$ decrease, preserving however the overall scaling relations in the limit of low salt and the approach to the universal asymptote at high salt (compare Fig. 5A and B). According to our adsorption criterion, eqn (10), longer chains will clearly accumulate the same binding energy for smaller $|\sigma|$. A similar behavior was observed for PE adsorption onto Janus particles:[59] the entire $\sigma_c(\kappa a)$ dependence shifts down for longer chains but preserves the scaling properties for small and large $\kappa a$ regimes.

In Fig. 5 flexible chains are considered, with the non-ES persistence length of $l_{p,0} \lesssim 10$ Å. For a spherical cavity, the theoretical results of ref. 39 for $\sigma_c$ give an excellent agreement with the results of our simulations for $N$ = 100 chains if we set $b = 2l_{p,0} \approx 4$ Å, a realistic value for flexible chains simulated. This follows from eqn (7) for PEs inside spherical cavities for $\kappa a \ll 1$ from which the critical charge density can be recalculated in units C m$^{-2}$ as

$$\frac{\sigma_c^{\rm sp,inv}}{\rm C\ m^{-2}} = 3C^2\frac{16br_0}{24\pi a^3 l_B} \approx 1.9\times10^{-5}. \qquad (12)$$

The same Kuhn length $b$ is then used to compute the full $\sigma_c^{\rm inv}(\kappa)$ asymptotes from the theoretically predicted[39] relations for $\delta_c^{\rm cyl,inv}(\kappa)$ and $\delta_c^{\rm pl,inv}(\kappa)$, according to eqn (1).

Due to the adsorption criterion implemented, for $N$ = 20 chains $\sigma_c$ is nearly 100/20 = 5 times larger than for $N$ = 100 polymers (compare the panels in Fig. 5 and see also the universal curves in Fig. 7). Also note that for $\kappa a \gg 1$ our simulations of the PE adsorption under confinement yield the $\sigma_c(\kappa) \sim \kappa^3$ scaling behavior, as anticipated for polymers with a salinity-independent Kuhn length $b$.[17] This is in contrast for instance to PE adsorption on the outside of spherical particles, where the effects of ES persistence are important and our simulations in the high-salt limit give $\sigma_c(\kappa) \sim \kappa^{1.9}$ scaling instead (see Fig. 8A in ref. 59).

We also examined the dependence of the critical adsorption conditions for semiflexible chains in all three adsorption geometries (see Fig. 6 and 10). Fig. 10 shows that for more persistent chains the magnitude of $|\sigma_c|$ decreases for the adsorption onto the planar slit, inside a cylindrical pore, and inside spherical cavities. We find that particularly for PE adsorption inside spherical cavities the magnitude $|\sigma_c|$ decreases due to a bending-energy driven localization of polymers near the cavity surface (see Fig. 6), which is particularly pronounced for the chains much longer than the cavity dimensions (see also ref. 99). For PE-sphere inverted adsorption, stiffer PEs prefer to stay closer to the adsorbing interface thus reducing the value of $|\sigma_c|$. The precise behavior of $\sigma_c$ as a function of $\kappa a$ shows that the deviations from the flexible chain

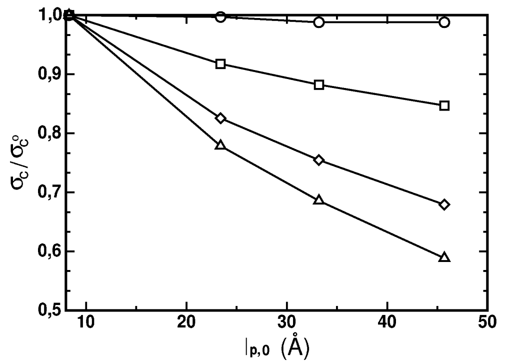


Fig. 6 Critical adsorption charge density for persistent *versus* flexible polymers inside a spherical cavity, $\sigma_c/\sigma_c^0$, computed for varying non-ES polymer persistence length. Parameters: $a$ = 50 Å, $N$ = 100, $\kappa a$ = 1 (circles), 5 (squares), 8 (diamonds) and 10 (triangles).

 This journal is © The Royal Society of Chemistry 2015

Published on 22 April 2015. Downloaded by UNIVERSITATSBIBLIOTHEK POTSDAM on 27/05/2015 10:41:52.

results become progressively larger for more persistent chains and at larger $\kappa a$ values (see Fig. 6). The latter is not surprising because at high-salt conditions the ES contribution to the polymer persistence gets reduced and the PE stiffness is dominated by its mechanical part $l_{p,0}$ (see eqn (11)).

The question arises whether for inverted PE critical adsorption the variation of the confinement degree or salt concentration gives rise to different $\sigma_c(\kappa a)$ behaviors. We showed that for adsorption of finite-length PEs onto spherical Janus particles[59] there was no universal parameter $\kappa a$ that would combine the curvature and salinity effects on the critical adsorption properties $\sigma_c(\kappa a)$. The inverted critical PE adsorption is also quite different if one varies the size of the confined cavities, tubes, and slits or the solution salinity (compare the curves in Fig. 11 for spherical confinement). Longer chains require smaller surface charge densities to get adsorbed and for smaller sizes of spherical cavities the value of $\sigma_c$ increases. This can be understood from the variation of the ES surface potential in spherical cavities presented in Fig. 2B showing that $\Psi(a) \approx 2(\kappa a)e_0\varphi(a)/(k_BT) \sim \kappa a$ for $\kappa a \ll 1$.[39] For inverted critical PE adsorption we obtain that indeed there exists no universal parameter $\kappa a$. This at first sight disagrees with the theoretical results of ref. 39. For the finite-length PEs with varying ES persistence studied in our simulations this disagreement is however not surprising, as compared to infinitely long flexible salt-insensitive polymers studied in the theoretical idealization.[5,39]

Fig. 7 illustrates the behavior of the rescaled critical surface charge density for inverted PE-sphere adsorption, $\sigma_c aN$. This combination accounts for the peculiar features of the variation of the ES potential with the cavity radius (Fig. 2B) and the adsorption condition used in the simulations (eqn (10)). We find a universal collapse of this renormalized parameter for the critical adsorption curves for different chain lengths and cavity sizes, for a wide range of variation of the solution salinity. We finally note that the adsorption criterion (10) was used throughout the paper. The inset of Fig. 10 illustrates however the behavior of PE adsorption–desorption boundary $\sigma_c(\kappa)$ onto spherical cavities if the criterion of $k_BT/10$ average binding energy per monomer is used. We find that the functional dependence of $\sigma_c(\kappa)$ obtained with such a criterion also agrees with theoretical predictions.[39]

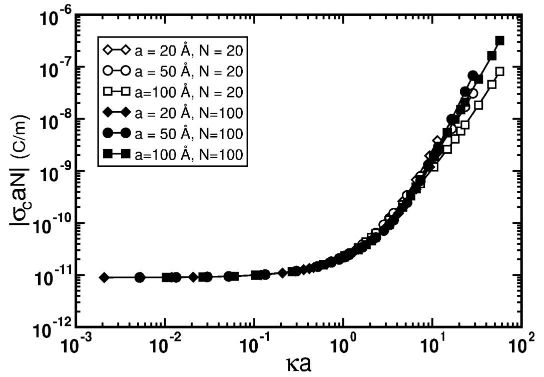


Fig. 7 Universal rescaled surface charge density for critical PE adsorption inside spherical cavities of varying radii and for polymers of different lengths, plotted for varying $\kappa$; $l_{p,0}$ = 8 Å.

# IV. Discussion

In this study, we have employed extensive Monte-Carlo computer simulations to unveil the physical properties of PE adsorption in confined spaces, considering polymer chains inside a planar slit, a cylindrical pore, and a spherical cavity. We rationalized the position of the adsorption–desorption transition upon variation of various physical parameters such as the extent of the external confinement, the salinity of the solution, the chain length, and the bare persistence length of the polymer. We have demonstrated how the well-known cubic scaling of the critical surface charge density with the reciprocal Debye screening length $\kappa$ gets non-trivially modified. Namely, in the limit of $\kappa a \ll 1$—small solution salinities or large surface curvature $1/a$—for the critical adsorption condition for PEs under confinement splits for the three fundamental geometries. We illustrate this behavior in Fig. 5 which is the main result of this study. Our results revealed a remarkable quantitative agreement with the recent theoretical predictions for the same system.[39] The simulation approach enabled us to vary the polymer length and PE persistence, which are often quite problematic to be properly implemented from the first theoretical principles.[18] Also, we showed that for the critical adsorption onto concave surfaces more persistent chains require smaller surface charge densities to get adsorbed. For critical adsorption of PEs of varying polymerization degree $N$ inside spherical cavities of radius $a$, we found that the simulation results collapse onto a universal curve if the rescaled surface charge density is considered, namely $\sigma_c \rightarrow \sigma_c aN$.

Finally, only the static properties of PEs under confinement were considered in the current paper. It would be instructive as a next step to study the dynamics of charged polyions inside oppositely charged domains and cavities. In particular, the implications of polymer charge and adsorption to the interior of the spherical cavity can enrich the trends observed for looping kinetics of spherically confined flexible and semi-flexible chains.[99] The video files of the Supplementary material we present here demonstrate, for instance, that the dynamics of PE chains in the adsorbed state is slowed down dramatically, as compared to desorbed configurations. This surface-mediated polymer confinement is consistent with the ultraslow relaxation of confined DNA molecules detected in single-molecule experiments during viral packaging.[119] Future developments of the model will include the study of PE adsorption onto pH-responsive functionalized[120] curved surfaces, the implications of a nonlinear ES potential distribution for the position of the adsorption–desorption boundary $\sigma_c(\kappa,N)$,[113] and the adsorption of polymer chains with heterogeneous charge distribution. The latter can be applied, for instance, to the surface-mediated adsorption of polypeptide chains of partially folded proteins.

Let us discuss some possible applications of our findings. Polymer encapsidation inside oppositely charged cavities[42,70,77,96,121,122] is the fundamental mechanism of assembly of cylindrical and spherical single-stranded RNA viruses.[89,90] This process employs a delicately tuned adsorption of negatively charged RNA chains onto the positively charged

interior of viral protein shells. Direct applications of our observations to the properties of real RNA viruses might however require the secondary RNA looped structure to be taken into account. The latter often plays an important role in the viral assembly and nucleic acid packaging process.[42,123] Branching and self-association in the structure of compacted RNA yield, for instance, a weak overcharging of the entire virion: on average the negative charge of the enclosed nucleic acid chain is about 1.6 times larger than the positive charge of the enveloping protein shell.[29] Also note that a low dielectric permittivity of viral protein shells can affect the association of single-stranded DNA chains on the interior of capsid surfaces.[94–96] Here, there exist some theoretical[84] and simulation-based[85] predictions for the effects of dielectric continuities on weak PE–surface adsorption. The confined weak PE adsorption onto low-dielectric surfaces has not yet been studied so far, to the best of our knowledge. This can be an interesting subject for future investigations.[113]

Another domain of possible applications includes the behavior of long DNA molecules in micro-fluidic devices involving nano-channels[124–127] with attractive walls. Having in mind some applications to cylindrical channels of non-trivial cross-section,[128] one can consider in the future the PE adsorption on the interior of tubes with more complicated geometries, *e.g.* rectangular or triangular rather than circular cylindrical channels. Some applications of our findings to the description of charge effects of PE and DNA translocation through natural and synthetic nano-pores[129] are also possible. Another interesting issue is the lateral diffusion of polymers along transiently adsorbing interfaces[130,131] where clear subdiffusive features for the chain displacement were measured in recent single-molecule tracking experiments;[132] see also ref. 133. Related to these translocation and surface diffusion issues is the problem of PE deposition and critical polymer–surface adsorption under externally applied shear and in the presence of hydrodynamic interactions.[134,135]

One more immediate application of our results includes the problems of protein adsorption—both in their native form and in the denatured state—in various porous media. For instance, polymer dynamics and adsorption in sticky nano-channels of porous silicon studied in ref. 136 can pave the way for the selective separation of proteins from unknown mixtures, based on their surface charge and surface–adsorption properties. Moreover, defining the critical adsorption conditions is of vital importance for the fabrication of responsive and permeable multilayer capsids. They are being formed *via* the alternating adsorption of oppositely charged PEs[7] and used for diagnostic and therapeutic purposes.[137] Finally, nano-structured polymer-functionalized porous materials are used in electro-chemical super-capacitors[138,139] and our results on polymers under extreme confinement might find some future applications in this area as well.

## Appendix A: additional figures

In this appendix we present the additional Fig. 8–11 which support the claims in the main text of the manuscript.

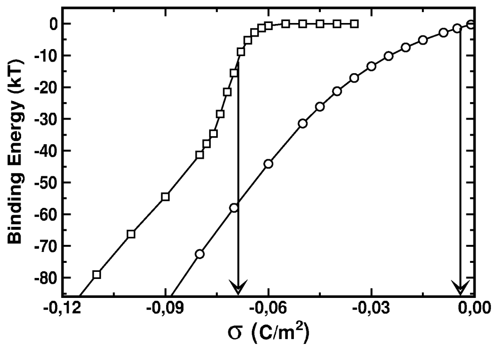


Fig. 8 The variation of PE binding energy with the surface charge density. For a polymer adsorbing onto an oppositely charged sphere a sharp transition in the average binding energy exists. This indicates a first-order-like transition, realized in computer simulations of weak PE adsorption onto oppositely charged spheres[64] and rods.[61] In contrast, for a PE chain inside a spherical cavity the $E_b(\sigma)$ variation is smooth in the whole range of surface charge densities, including the critical adsorption point at $\sigma = \sigma_c$. The arrows indicate the values of the corresponding critical surface charge densities, as obtained with two different adsorption criteria (see the main text for details). Parameters: $N = 100$ and $\kappa a = 10$.

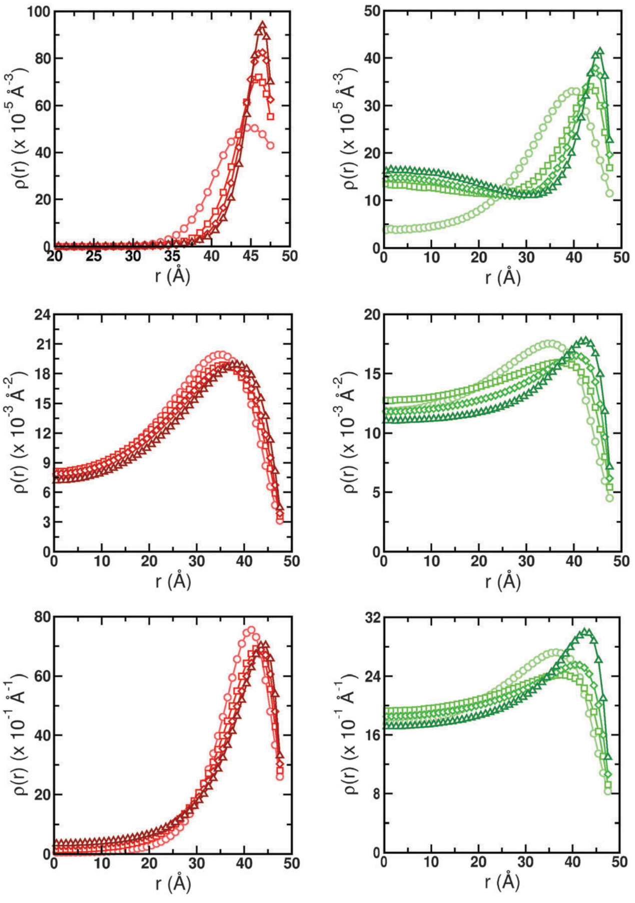


Fig. 9 Distribution of semi-flexible polymers inside a spherical cavity (top), cylindrical pore (middle) and planar slit (bottom panels) for the parameters of Fig. 3 and for $N = 100$, $\kappa a = 0.5$ (left panels, reddish colors) and $\kappa a = 5.0$ (right panels, greenish colors). The color scheme matches that of Fig. 3. The non-ES persistent length is $l_{p,0} = 8$ (circles), 23 (squares), 33 (diamonds) and 46 Å (triangles).

Published on 22 April 2015. Downloaded by UNIVERSITATSBIBLIOTHEK POTSDAM on 27/05/2015 10:41:52.

View Article Online


Published on 22 April 2015. Downloaded by UNIVERSITATSBIBLIOTHEK POTSDAM on 27/05/2015 10:41:52.

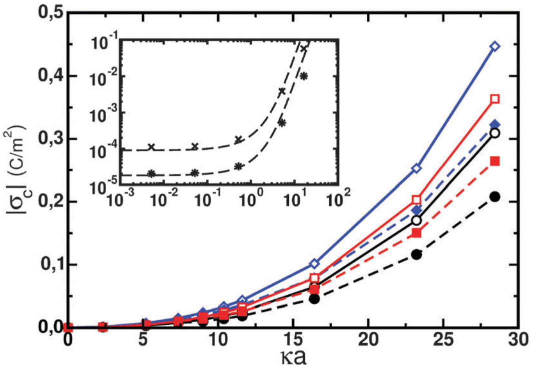


Fig. 10 The main figure shows the same as in Fig. 5 for inverted adsorption inside a spherical cavity (black), cylindrical tube (red), and planar slit (blue symbols) for varying salt conditions $\kappa$. The results are plotted in the linear scale. The polymer stiffness is $l_{p,0}$ = 8 Å (open symbols) and $l_{p,0}$ = 50 Å (full symbols). Parameters for the main figure: $a$ = 54 Å and $N$ = 20. The inset is the critical charge density for a spherical cavity as obtained based on the adsorption criterion of $k_BT/10$ average binding energy per monomer. The results for flexible PE chains ($l_{p,0}$ = 8 Å) with $N$ = 20 and $N$ = 100 monomers are shown respectively as crosses and stars in the inset. The theoretical prediction for the functional dependence of $\sigma_c(\kappa)$ is represented by dashed curves, plotted according to eqn (5)–(7) in ref. 39 and adjusted vertically to fit the simulation data.

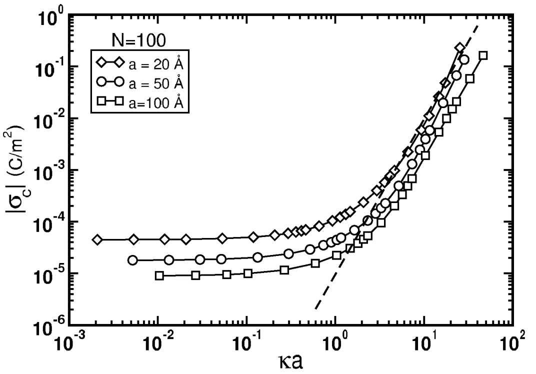


Fig. 11 The same as in Fig. 5 but for varying radius $a$ of the spherical cavities. The high-salt asymptote (8) for the charge density (in units of C m$^{-2}$) is obtained from eqn (8) as $\sigma_c(\kappa)/[\mathrm{C\ m^{-2}}] = C^2\kappa^3 b r_0/(\pi l_B) \sim \kappa^3$ (the dashed line). Parameters: $N$ = 100, $a$ = 50 Å, $l_{p,0}$ = 8 Å.

## Appendix B: supplementary material

In the Supplementary material we include the video files illustrating the change of polymer conformations for the two basic geometries, as investigated in the main text. For each geometry, we fix the value of the surface charge density $\sigma$ and the confinement dimensions $a$ and vary the solution salinity. In doing so, at small $\kappa a$ values the polyelectrolyte chain is rather in the adsorbed state, while for larger $\kappa a$ the electrostatic polymer–surface screening gets stronger, the system crosses the adsorption–desorption boundary, and the chain desorbs from the interface (see also Fig. 6 of the main text). Parameters: the spherical cavity with a surface charge density of $\sigma = -0.1/(4\pi)$ C m$^{-2}$, the sphere radius is $a$ = 50 Å, and the chain polymerization degree is $N$ = 100, simulated at $\kappa a$ = 1 (Video 1, ESI†) and 10 (Video 2, ESI†). The cylindrical pore for the same values of $\sigma$, $N$, and $a$ simulated for $\kappa a$ = 1 (Video 3, ESI†) and 10 (Video 4, ESI†). The polyelectrolyte adsorption inside planar slits for the same $\sigma$, $N$, and the slab thickness of $a$ = 100 Å was simulated for $\kappa a$ = 1 (Video 5, ESI†) and 10 (Video 6, ESI†). Every video contains about $10^6$ elementary simulation steps. Note that the length of the trace shown is about 0.1 of the entire trajectory length used in Fig. 5 to determine the adsorption–desorption boundary.

## Acknowledgements

Computer resources were supplied by the Center for Scientific Computing (NCC/GridUNESP) of the Sao Paulo State University. The authors acknowledge funding from the Academy of Finland (FiDiPro scheme to RM) and the German Research Foundation (DFG Grant CH 707/5-1 to AGC).

## References


1 R. R. Netz and D. Andelman, Neutral and Charged Polymers at Interfaces, *Phys. Rep.*, 2003, **380**, 1.

2 A. V. Dobrynin and M. Rubinstein, Theory of Polyelectrolytes in Solutions and at Surfaces, *Prog. Polym. Sci.*, 2005, **30**, 1049.

3 I. M. Lifshitz, A. Yu. Grosberg and A. R. Khokhlov, Some Problems of the Statistical Physics of Polymer Chains with Volume Interaction, *Rev. Mod. Phys.*, 1978, **50**, 683.

4 A. V. Dobrynin, Theory and Simulations of Charged Polymers: From Solution Properties to Polymeric Nanomaterials, *Curr. Opin. Coll. Interf. Sci.*, 2008, **13**, 376.

5 R. G. Winkler and A. G. Cherstvy, Strong and Weak Polyelectrolyte Adsorption onto Oppositely Charged Curved Surfaces, *Adv. Polym. Sci.*, 2014, **255**, 1.

6 M. A. Cohen Stuart, *et al.*, Emerging Applications of Stimuli-Responsive Polymer Materials, *Nature Mat.*, 2010, **9**, 101.

7 A. A. Antipov and G. B. Sukhorukov, Polyelectrolyte Multilayer Capsules as Vehicles with tunable Permeability, *Adv. Coll. Interf. Sci.*, 2004, **111**, 49.

8 H. Tanaka, *Paper*, Dekker, New York, 1998, ch. 19.

9 T. Lindström, in *Paper Chemistry*, ed. J. C. Roberts, Blackie, London, 1991, p. 25.

10 A. Takahashi and M. Kawaguchi, The Structure of Macromolecules Adsorbed on Interfaces, *Adv. Polym. Sci.*, 1982, **46**, 1.

11 T. Humplik, *et al.*, Nanostructured Materials for Water Desalination, *Nanotechnology*, 2011, **22**, 292001.

12 F. Fadhillah, *et al.*, Development of Polyelectrolyte Multilayer thin Film Composite Membrane for Water Desalination Application, *Desalination*, 2013, **318**, 19.

13 S. S. Patel and M. Tirrell, Measurement of Forces Between Surfaces in Polymer Fluids, *Annu. Rev. Phys. Chem.*, 1989, **40**, 597.

Published on 22 April 2015. Downloaded by UNIVERSITATSBIBLIOTHEK POTSDAM on 27/05/2015 10:41:52.

14 I. Szilagyi, G. Trefalt, A. Tiraferri, P. Maroni and M. Borkovec, Polyelectrolyte Adsorption, Interparticle Forces, and Colloidal Aggregation, *Soft Matter*, 2014, **10**, 2479.
15 P.-G. de Gennes, Flexible Polymers in Nanopores, *Adv. Polym. Sci.*, 1999, **138**, 91.
16 S. Napolitano and M. Wübbenhorst, The Lifetime of the Deviations from Bulk Behaviour in Polymers Confined at the Nanoscale, *Nature Comm.*, 2011, **2**, 260.
17 F. W. Wiegel, Adsorption of a Macromolecule to a Charged Surface, *J. Phys. A*, 1977, **10**, 299.
18 M. Muthukumar, Adsorption of a Polyelectrolyte Chain to a Charged Surface, *J. Chem. Phys.*, 1987, **86**, 7230.
19 F. von Goeler and M. Muthukumar, Adsorption of Polyelectrolytes onto Curved Surfaces, *J. Chem. Phys.*, 1994, **100**, 7796.
20 G. S. Manning, Counterion Condensation on Charged Spheres, Cylinders, and Planes, *J. Phys. Chem. B*, 2007, **111**, 8554.
21 R. G. Winkler, M. Gold and P. Reineker, Collapse of Polyelectrolyte Macromolecules by Counterion Condensation and Ion Pair Formation: A Molecular Dynamics Simulation Study, *Phys. Rev. Lett.*, 1998, **80**, 3731.
22 H. Schiessel, The Physics of Chromatin, *J. Phys.: Condens. Matter*, 2003, **15**, R699.
23 R. R. Netz and J. F. Joanny, Adsorption of semiflexible polyelectrolytes on charged planar surfaces: charge compensation, charge reversal, and multilayer formation, *Macromolecules*, 1999, **32**, 9013.
24 K. K. Kunze and R. R. Netz, Salt-Induced DNA-Histone Complexation, *Phys. Rev. Lett.*, 2000, **85**, 4389.
25 E. Gurovitch and P. Sens, Adsorption of Polyelectrolyte onto a Colloid of Opposite Charge, *Phys. Rev. Lett.*, 1999, **82**, 339.
26 A. Shafir, D. Andelman and R. R. Netz, Adsorption and Depletion of Polyelectrolytes from Charged Surfaces, *J. Chem. Phys.*, 2003, **119**, 2355.
27 A. Shafir and D. Andelman, Polyelectrolyte Adsorption: Chemical and Electrostatic Interactions, *Phys. Rev. E*, 2004, **70**, 061804.
28 A. Shafir and D. Andelman, Phase Behavior of Polyelectrolyte-Surfactant Complexes at Planar Surfaces, *Phys. Rev. E*, 2006, **74**, 021803.
29 V. A. Belyi and M. Muthukumar, Electrostatic Origin of the Genome Packing in Viruses, *Proc. Natl. Acad. Sci. U. S. A.*, 2006, **103**, 17174.
30 H. Boroudjerdi, A. Naji and R. R. Netz, Global Analysis of the Ground-State Wrapping Conformation of a Charged Polymer on an Oppositely Charged Nano-Spheres, *Europ. Phys. J. E*, 2014, **37**, 21.
31 M. Muthukumar, Polymers under Confinement, *Adv. Chem. Phys.*, 2012, **149**, DOI: 10.1002/9781118180396.ch4.
32 M. Muthukumar, Pattern Recognition by Polyelectrolytes, *J. Chem. Phys.*, 1995, **103**, 4723.
33 T. A. Kampmann, H. H. Boltz and J. Kierfeld, Controlling Adsorption of Semiflexible Polymers on Planar and Curved Substrates, *J. Chem. Phys.*, 2013, **139**, 034903.
34 J. Forsman, Polyelectrolyte Adsorption: Electrostatic Mechanisms and Nonmonotonic Responses to Salt Addition, *Langmuir*, 2012, **28**, 5138.
35 R. G. Winkler and A. G. Cherstvy, Critical Adsorption of Polyelectrolytes onto Charged Spherical Colloids, *Phys. Rev. Lett.*, 2006, **96**, 066103.
36 A. G. Cherstvy and R. G. Winkler, Strong and Weak Adsorptions of Polyelectrolyte Chains onto Oppositely Charged Spheres, *J. Chem. Phys.*, 2006, **125**, 064904.
37 R. G. Winkler and A. G. Cherstvy, Adsorption of Weakly Charged Polyelectrolytes onto Oppositely Charged Spherical Colloids, *J. Phys. Chem. B*, 2007, **111**, 8486.
38 A. G. Cherstvy and R. G. Winkler, Polyelectrolyte Adsorption onto Oppositely Charged Interfaces: Unified Approach for Plane, Cylinder, and Sphere, *Phys. Chem. Chem. Phys.*, 2011, **13**, 11686.
39 A. G. Cherstvy, Critical Polyelectrolyte Adsorption under Confinement: Planar Slit, Cylindrical Pore, and Spherical Cavity, *Biopolymers*, 2012, **97**, 311.
40 A. Siber, A. L. Bozic and R. Podgornik, Energies and Pressures in Viruses: Contribution of Nonspecific Electrostatic Interactions, *Phys. Chem. Chem. Phys.*, 2012, **14**, 3746.
41 A. Siber and R. Podgornik, Nonspecific Interactions in Spontaneous Assembly of Empty *versus* Functional Single-Stranded RNA Viruses, *Phys. Rev. E*, 2008, **78**, 051915.
42 G. Erdemci-Tandogan, J. Wagner, P. van der Schoot, R. Podgornik and R. Zandi, RNA Topology remolds Electrostatic Stabilization of Viruses, *Phys. Rev. E*, 2014, **89**, 032707.
43 A. B. Kayitmazer, *et al.*, Protein-Polyelectrolyte Interactions, *Soft Matter*, 2013, **9**, 2553.
44 Y. G. Mishael, P. L. Dubin, R. de Vries and A. B. Kayitmazer, Effect of Pore Size on Adsorption of a Polyelectrolyte to Porous Glass, *Langmuir*, 2007, **23**, 2510.
45 C. L. Cooper, P. L. Dubin, A. B. Kayitmazer and S. Turksen, Polyelectrolyte-Protein Complexes, *Curr. Opin. Coll. Interf. Sci.*, 2005, **10**, 52.
46 K. R. Grymonpre, B. A. Staggemeier, P. L. Dubin and K. W. Mattison, Identification by integrated Computer Modeling and Light Scattering Studies of an Electrostatic Serum Albumin-Hyaluronic Acid Binding Site, *Biomacromolecules*, 2001, **2**, 422.
47 X. H. Feng, *et al.*, Critical Conditions for Binding of Dimethyldodecylamine Oxide Micelles to Polyanions of Variable Charge Density, *Macromolecules*, 2001, **34**, 6373.
48 N. Hansupalak and M. M. Santore, Sharp Polyelectrolyte Adsorption Cutoff Induced by a Monovalent Salt, *Langmuir*, 2003, **19**, 7423.
49 C. L. Cooper, *et al.*, Effects of Polyelectrolyte Chain Stiffness, Charge Mobility and Charge Sequences on Binding to Proteins and Micelles, *Biomacromolecules*, 2006, **7**, 1025.
50 E. Kizilay, A. B. Kayitmazer and P. L. Dubin, Complexation and Coacervation of Polyelectrolytes with Oppositely Charged Colloids, *Adv. Coll. Interf. Sci.*, 2011, **167**, 24.
51 Y. Wang, P. L. Dubin and H. Zhang, Interaction of DNA with Cationic Micelles: Effects of Micelle Surface Charge

 This journal is © The Royal Society of Chemistry 2015

Published on 22 April 2015. Downloaded by UNIVERSITATSBIBLIOTHEK POTSDAM on 27/05/2015 10:41:52.

Density, Micelle Shape, and Ionic Strength on Complexation and DNA Collapse, *Langmuir*, 2001, **17**, 1670.
52 M. Antonov, M. Mazzawi and P. L. Dubin, Entering and Exiting the Protein-Polyelectrolyte Coacervate Phase *via* Nonmonotonic Salt Dependence of Critical Conditions, *Biomacromolecules*, 2010, **11**, 51.
53 S. Sennato, D. Truzzolillo and F. Bordi, Aggregation and Stability of Polyelectrolyte-Decorated Liposome Complexes in Water-Salt Media, *Soft Matter*, 2012, **8**, 9384.
54 S. Sennato, L. Carlini, D. Truzzolillo and F. Bordi, arXiv:1503.02847.
55 A. A. Zinchenko, K. Yoshikawa and D. Baigl, Compaction of Single-Chain DNA by Histone-Inspired Nanoparticles, *Phys. Rev. Lett.*, 2005, **95**, 228101.
56 A. Poghossian, *et al.*, Electrical Monitoring of Polyelectrolyte Multilayer Formation by Means of Capacitive Field-Effect Devices, *Analyt. Bioanalyt. Chem.*, 2013, **405**, 6425.
57 J.-P. Chapel and J.-F. Berret, Versatile Electrostatic Assembly of Nanoparticles and Polyelectrolytes: Coating, Clustering and Layer-by-Layer Processes, *Curr. Opin. Coll. & Interf. Sci.*, 2012, **17**, 97.
58 I. V. Malyar, *et al.*, Photocontrolled Adsorption of Polyelectrolyte Molecules on a Silicon Substrate, *Langmuir*, 2013, **29**, 16058.
59 S. J. de Carvalho, R. Metzler and A. G. Cherstvy, Critical Adsorption of Polyelectrolytes onto Charged Janus Nanospheres, *Phys. Chem. Chem. Phys.*, 2014, **16**, 15539.
60 J. Shin, A. G. Cherstvy and R. Metzler, Sensing Viruses by Mechanical Tension of DNA in Responsive Hydrogels, *Phys. Rev. X*, 2014, **4**, 021002.
61 S. J. de Carvalho and D. L. Z. Caetano, Adsorption of Polyelectrolytes onto Oppositely Charged Cylindrical Macroions, *J. Chem. Phys.*, 2013, **138**, 244909.
62 S. C. C. Nunes, T. F. G. G. Cova and A. A. C. C. Pais, A New Perspective on Correlated Polyelectrolyte Adsorption: Positioning, Conformation, and Patterns, *J. Chem. Phys.*, 2013, **139**, 054906.
63 G. Luque-Caballero, A. Martin-Molina and M. Quesada-Perez, Polyelectrolyte Adsorption onto like-charged Surfaces mediated by trivalent Counterions: a Monte Carlo Simulation Study, *J. Chem. Phys.*, 2014, **140**, 174701.
64 S. J. de Carvalho, First-order-like Transition in Salt-induced Macroion-Polyelectrolyte Desorption, *EPL*, 2010, **92**, 18001.
65 V. M. de Oliveira and S. J. de Carvalho, Adsorption of pH-responsive Polyelectrolyte Chains onto Spherical Macroions, *Eur. Phys. J. E*, 2014, **37**, 75.
66 F. Carnal and S. Stoll, Adsorption of Weak Polyelectrolytes on Charged Nanoparticles. Impact of Salt Valency, pH, and Nanoparticle Charge Density: Monte-Carlo Simulations, *J. Phys. Chem. B*, 2011, **115**, 12007.
67 S. Ulrich, M. Seijo, F. Carnal and S. Stoll, Formation of Complexes between Nanoparticles and Weak Polyampholyte Chains. Monte Carlo Simulations, *Macromolecules*, 2011, **44**, 1661.
68 J.-M. Y. Carrillo and A. V. Dobrynin, Molecular Dynamics Simulations of Polyelectrolyte Adsorption, *Langmuir*, 2007, **23**, 2472.
69 T. Vogel and M. Bachmann, Conformational Phase Diagram for Polymers Adsorbed on Ultrathin Nanowires, *Phys. Rev. Lett.*, 2010, **104**, 198302.
70 J. Wang and M. Muthukumar, Encapsulation of a Polyelectrolyte Chain by an Oppositely Charged Spherical Surface, *J. Chem. Phys.*, 2011, **135**, 194901.
71 S. V. Lyulin, I. Vattulainen and A. A. Gurtovenko, Complexes Comprised of Charged Dendrimers, Linear Polyelectrolytes, and Counterions: Insight through Coarse-Grained Molecular Dynamics Simulations, *Macromolecules*, 2008, **41**, 4961.
72 Z. Wang, *et al.*, Charge Inversion by Flexible Polyelectrolytes on Spherical Surfaces: Numerical Self-Consistent Field Calculations under the Ground-State Dominance Approximation, *Macromolecules*, 2011, **44**, 8607.
73 S. Stoll and P. Chodanowski, Polyelectrolyte Adsorption on an Oppositely Charged Spherical Particle. Chain Rigidity Effects, *Macromolecules*, 2002, **35**, 9556.
74 A. Laguecir, *et al.*, Interactions of a Polyanion with a Cationic Micelle: Comparison of Monte Carlo Simulations with Experiment, *J. Phys. Chem. B*, 2003, **107**, 8056.
75 S. Ulrich, A. Laguecir and S. Stoll, Complexation of a Weak Polyelectrolyte with a Charged Nanoparticle. Solution Properties and Polyelectrolyte Stiffness Influences, *Macromolecules*, 2005, **38**, 8939.
76 R. de Vries, Monte Carlo Simulations of flexible Polyanions complexing with Whey Proteins at their Isoelectric Point, *J. Chem. Phys.*, 2004, **120**, 3475.
77 Q. Cao and M. Bachmann, Dynamics and Limitations of spontaneous Polyelectrolyte Intrusion into a charged Nanocavity, *Phys. Rev. E*, 2014, **90**, 060601(R).
78 J. Sheng and K. Luo, Conformation and adsorption transition on an attractive surface of a ring polymer in solution, *RSC Adv.*, 2015, **5**, 2056.
79 D. Andelman and J.-F. Joanny, On the Adsorption of Polymer Solutions on Random Surfaces: The Annealed Case, *Macromolecules*, 1991, **24**, 6040.
80 N. Hoda and S. Kumar, Theory of Polyelectrolyte Adsorption onto Surfaces Patterned with Charge and Topography, *J. Chem. Phys.*, 2008, **128**, 124907.
81 L. Li and S. Garde, Binding, Structure, and Dynamics of Hydrophobic Polymers near Patterned Self-Assembled Monolayer Surfaces, *Langmuir*, 2014, **30**, 14204.
82 M. Möddel, W. Janke and M. Bachmann, Adsorption and Pattern Recognition of Polymers at Complex Surfaces with Attractive Stripelike Motif, *Phys. Rev. Lett.*, 2014, **112**, 148303.
83 S. Srebnik, A. K. Chakraborty and E. I. Shakhnovich, Adsorption-Freezing Transition for Random Heteropolymers near Disordered 2D Manifolds due to "Pattern Matching", *Phys. Rev. Lett.*, 1996, **77**, 3157.
84 A. G. Cherstvy and R. G. Winkler, Polyelectrolyte Adsorption onto Oppositely Charged Interfaces: Image-Charge Repulsion and Surface Curvature, *J. Phys. Chem. B*, 2012, **116**, 9838.
85 M. Seijo, M. Pohl, S. Ulrich and S. Stoll, Dielectric discontinuity effects on the adsorption of a linear polyelectrolyte at the

View Article Online


Published on 22 April 2015. Downloaded by UNIVERSITATSBIBLIOTHEK POTSDAM on 27/05/2015 10:41:52.


surface of a neutral nanoparticle, *J. Chem. Phys.*, 2009, **131**, 174704.

86 R. Messina, Effect of image forces on polyelectrolyte adsorption, *Phys. Rev. E*, 2004, **70**, 0518021.

87 C. Forrey and M. Muthukumar, Electrostatics of capsid-induced viral RNA Organization, *J. Chem. Phys.*, 2009, **131**, 105101.

88 E. C. Dykeman, P. G. Stockley and R. Twarock, Solving a Levinthal's Paradox for Virus Assembly identifies a unique Antiviral Strategy, *Proc. Natl. Acad. Sci. U. S. A.*, 2014, **111**, 5361.

89 J. D. Perlmutter, M. R. Perkett and M. F. Hagan, Pathways for Virus Assembly around Nucleic Acids, *J. Mol. Biol.*, 2014, **426**, 3148.

90 M. F. Hagan, Modeling Viral Capsid Assembly, *Adv. Chem. Phys.*, 2014, 155, ch. 1; arXiv:1301.1657.

91 A. Klug, The Tobacco Mosaic Virus Particle: Structure and Assembly, *Phil. Trans. R. Soc. Lond. B*, 1999, **354**, 531.

92 R. D. Cadena-Nava, *et al.*, Self-Assembly of Viral Capsid Protein and RNA Molecules of Different Sizes: Requirement for a Specific High Protein/RNA Mass Ratio, *J. Virol.*, 2012, **86**, 3318.

93 Y. Hu, R. Zandi, A. Anavitarte, C. M. Knobler and W. M. Gelbart, Packaging of a Polymer by a Viral Capsid: The Interplay between Polymer Length and Capsid Size, *Biophys. J.*, 2008, **94**, 1428.

94 A. Cuervo, *et al.*, Direct Measurement of the Dielectric Polarization Properties of DNA, *Proc. Natl. Acad. Sci. U. S. A.*, 2014, **111**, E3624.

95 C. N. Schutz and A. Warshel, What are the dielectric "constants" of proteins and how to validate electrostatic models?, *Proteins*, 2001, **44**, 400.

96 A. G. Cherstvy, Electrostatic Interactions in Biological DNA-Related Systems, *Phys. Chem. Chem. Phys.*, 2011, **13**, 9942.

97 A. Akinchina and P. Linse, Monte Carlo Simulations of Polyion-Macroion Complexes. 1. Equal Absolute Polyion and Macroion Charges, *Macromolecules*, 2002, **35**, 5183.

98 B. O'Shaughnessy and D. Vavylonis, Irreversibility and Polymer Adsorption, *Phys. Rev. Lett.*, 2003, **90**, 056103.

99 J. Shin, A. G. Cherstvy and R. Metzler, Polymer Looping Is Controlled by Macromolecular Crowding, Spatial Confinement, and Chain Stiffness, *ACS Macro Lett.*, 2015, **4**, 202.

100 P. Vazquez-Montejo, Z. McDargh, M. Deserno and J. Guven, *Cylindrical Confinement of Semiflexible Polymers*, arXiv:1503.01023.

101 L. Schefer, I. Usov and R. Mezzenga, Anomalous Stiffening and Ion-Induced Coil-Helix Transition of Carrageenans in Monovalent Salt Conditions, *Biomacromolecules*, 2015, **16**, 985.

102 T. Odijk, Polyelectrolytes near the Rod Limit, *J. Polym. Sci. Polym. Phys. Ed.*, 1977, **15**, 477.

103 J. Skolnick and M. Fixman, Electrostatic Persistence Length of a Wormlike Polyelectrolyte, *Macromolecules*, 1977, **10**, 944.

104 A. G. Cherstvy, Effect of a low-dielectric Interior on DNA Electrostatic Response to Twisting and Bending, *J. Phys. Chem. B*, 2007, **111**, 12933.

105 R. Everaers, A. Milchev and V. Yamakov, The electrostatic persistence length of polymers beyond the OSF limit, *Eur. Phys. J. E*, 2002, **8**, 3.

106 D. Marenduzzo, *et al.*, DNA-DNA Interactions in Bacteriophage Capsids are responsible for the observed DNA Knotting, *Proc. Natl. Acad. Sci. U. S. A.*, 2009, **106**, 22269.

107 R. M. Fuoss, A. Katchalsky and S. Lifson, The Potential of an Infinite Rod-Like Molecule and the Distribution of the Counter Ions, *Proc. Natl. Acad. Sci. U. S. A.*, 1951, **37**, 579.

108 A. G. Cherstvy, Electrostatics of DNA Complexes with Cationic Lipid Membranes, *J. Phys. Chem. B*, 2007, **111**, 7914.

109 F. Fogolari, A. Brigo and H. Molinari, The Poisson–Boltzmann Equation for Biomolecular Electrostatics: a Tool for Structural Biology, *J. Mol. Recognit.*, 2002, **15**, 377.

110 C. Fleck and H. H. von Grünberg, Counterion Evaporation, *Phys. Rev. E*, 2001, **63**, 061804.

111 K. Wagner, D. Harries, S. May, V. Kahl, J. O. Rädler and A. Ben-Shaul, Direct evidence for counterion release upon cationic lipid-DNA condensation, *Langmuir*, 2000, **16**, 303.

112 D. Harries, S. May and A. Ben-Shaul, Counterion release in membrane-biopolymer interactions, *Soft Matter*, 2013, **9**, 9268.

113 S. J. de Carvalho, *et al.*, work in preparation.

114 R. Metzler, J.-H. Jeon, A. G. Cherstvy and E. Barkai, Anomalous Diffusion Models and their Properties: Non-stationarity, Non-ergodicity, and Ageing at the Centenary of Single Particle Tracking, *Phys. Chem. Chem. Phys.*, 2014, **16**, 24128.

115 J. Shin, A. G. Cherstvy and R. Metzler, Mixing and Segregation of Ring Polymers: Spatial Confinement and Molecular Crowding Effects, *New J. Phys.*, 2014, **16**, 053047.

116 B.-Y. Ha and Y. Jung, Polymers under Confinement: Single Polymers, how they interact, and as Model Chromosomes, *Soft Matter*, 2015, **11**, 2333.

117 M. A. Cohen Stuart, C. W. Hoogendam and A. de Keize, Kinetics of Polyelectrolyte Adsorption, *J. Phys.: Condens. Matter*, 1997, **9**, 7767.

118 P. Frantz and S. Granick, Kinetics of Polymer Adsorption and Desorption, *Phys. Rev. Lett.*, 1991, **66**, 899.

119 Z. T. Berndsen, *et al.*, Nonequilibrium Dynamics and ultraslow Relaxation of Confined DNA during Viral Packaging, *Proc. Natl. Acad. Sci. U. S. A.*, 2014, **111**, 8345.

120 E. Wischerhoff, N. Badi, J. F. Lutz and A. Laschewsky, Smart Bioactive Surfaces, *Soft Matter*, 2010, **6**, 705.

121 O. M. Elrad and M. F. Hagan, Encapsulation of a Polymer by an Icosahedral Virus, *Phys. Biol.*, 2010, **7**, 045003.

122 G. Saper, *et al.*, Effect of capsid confinement on the chromatin organization of the SV40 minichromosome, *Nucl. Acids Res.*, 2013, **41**, 1569.

123 R. Zandi and P. van der Schoot, Size Regulation of ss-RNA Viruses, *Biophys. J.*, 2009, **96**, 9.

124 Y.-L. Chen, M. D. Graham, J. J. de Pablo, G. C. Randall, M. Gupta and P. S. Doyle, Conformation and Dynamics of


 This journal is © The Royal Society of Chemistry 2015

Single DNA Molecules in Parallel-Plate Slit microchannels, *Phys. Rev. E*, 2004, **70**, 060901(R).
125 C. Manneschi, *et al.*, Stretching of DNA Confined in Nanochannels with Charged Walls, *Biomicrofluidics*, 2014, **8**, 064121.
126 W. Reisner, J. N. Pedersen and R. H. Austin, DNA Confinement in Nanochannels: Physics and Biological Applications, *Rep. Prog. Phys.*, 2012, **75**, 106601.
127 J. R. C. van der Maarel, C. Zhang and J. A. van Kan, A Nanochannel Platform for Single DNA Studies: From Crowding, Protein DNA Interaction, to Sequencing of Genomic Information, *Isr. J. Chem.*, 2014, **54**, 1573.
128 C. Manneschi, *et al.*, Conformations of DNA in Triangular Nanochannels, *Macromolecules*, 2013, **46**, 4198.
129 V. V. Palyulin, T. Ala-Nissila and R. Metzler, Polymer Translocation: the first two Decades and the recent Diversification, *Soft Matter*, 2014, **10**, 9016.
130 C. Yu, *et al.*, Single-Molecule Observation of Long Jumps in Polymer Adsorption, *ACS Nano*, 2013, **7**, 9735.
131 M. J. Skaug, J. N. Mabry and D. K. Schwartz, Single-Molecule Tracking of Polymer Surface Diffusion, *J. Am. Chem. Soc.*, 2014, **136**, 1327.
132 D. Wang, C. He, M. P. Stoykovich and D. K. Schwartz, Nanoscale Topography Influences Polymer Surface Diffusion, *ACS Nano*, 2015, **9**, 1656.
133 V. G. Guimaraes, *et al.*, Unusual diffusing Regimes Caused by Different Adsorbing Surfaces, *Soft Matter*, 2015, **11**, 1658.
134 N. Hoda and S. Kumar, Brownian dynamics simulations of polyelectrolyte adsorption in shear flow with hydrodynamic interaction, *J. Chem. Phys.*, 2007, **127**, 234902.
135 S. Dutta, K. D. Dorfman and S. Kumar, Shear-Induced Desorption of Isolated Polymer Molecules from a Planar Wall, *ACS Macro Lett.*, 2015, **4**, 271.
136 A. Kusmin, *et al.*, Polymer Dynamics in Nanochannels of Porous Silicon: A Neutron Spin Echo Study, *Macromolecules*, 2010, **43**, 8162.
137 B. G. de Geest, *et al.*, Polyelectrolyte Microcapsules for Biomedical Applications, *Soft Matter*, 2009, **5**, 282.
138 C. Meng, C. Liu, L. Chen, C. Hu and S. Fan, Highly Flexible and All-Solid-State Paperlike Polymer Supercapacitors, *Nano Lett.*, 2010, **10**, 4025.
139 P. Simon and Y. Gogotsi, Materials for Electrochemical Capacitors, *Nature Mat.*, 2008, **7**, 845.

Published on 22 April 2015. Downloaded by UNIVERSITATSBIBLIOTHEK POTSDAM on 27/05/2015 10:41:52.
